# Supplementary material for: Generalizable and Scalable Multistage Biomedical Concept Normalization Leveraging Large Language Models
Source: arXiv:2405.15122 source file (2024-05-24)
Supplement: Supplementary file 2 [file cover_letter.tex]

Nicholas J Dobbins
Assistant Professor
Biomedical Informatics \& Data Science Section, Dept. of Medicine
Johns Hopkins University
Baltimore, MD 21205-1832
nic.dobbins@jhu.edu


May 23, 2024 


Dr. Isaac Kohane
Editor-in-Chief
NEJM AI


Dear Dr. Kohane,

I am pleased to submit an original research article entitled "Generalizable and Scalable Multistage Biomedical Concept Normalization Leveraging Large Language Models" to be considered for publication in the New England Journal of Medicine - Artificial Intelligence.

This manuscript explores the integration of Large Language Models with existing rule-based UMLS concept normalization systems to improve biomedical concept normalization performance on clinical documents. We use an existing large publicly available dataset and two models - one proprietary and one open-source - and systematically evaluate both across 2 tasks: (1) synonym and alternate phrasing generation (improving recall) and (2) candidate concept pruning (improving precision). Our results demonstrate that when used in concert with existing widely-used normalization software, comparatively small and non-fine-tuned models can nonetheless significantly improve normalization performance. Our findings are particularly important given the ubiquity of the task of normalizing biomedical concepts in large corpora of documents, particularly when gold-standard data are unavailable or fine-tuning is not possible. This work advances biomedical normalization research and contributes to our understanding of practical methods and empirical model evaluation informing a wide variety of potential future research. 

This manuscript has not been previously published and is not under consideration elsewhere. We have no conflicts of interest to disclose. Thank you for your consideration.

Sincerely,

Nicholas J Dobbins
